# Supplementary material for: Domain Adaptive Decision Trees: Implications for Accuracy and Fairness
Source: arXiv:2302.13846 source file (2023-05-31)
Supplement: Supplementary file 1 [file Appendix.tex]

\section{Further Notes on Entropy}

\subsection{The Inherent Weight in the Information Gain}
\label{appendix:WeightOrigin}

From $IG$ \eqref{eq:BasicIG}, the \textit{weight term} $P(x)$ comes from the fact that we are taking the expectation of a function of a random variable. By the definition of expectation, recall that for $\mathbf{E}[\rho(X)]$, where $X$ is a random variable and $\rho$ a real-valued function, we have $\mathbf{E}[\rho(X)] = \sum_{x \in X}P(x)\rho(x)$. Notice that $H(\varphi|X=x)$ is not a random variable in itself but an output of a function of the random variable $X$: $\rho(X)=H(\varphi|X=x)$. To obtain the random variable $H(\varphi|X)$, we need to aggregate over all possible values of $X$, which we can do by taking its expectation over $\rho(X)$. This reasoning is what gives the standard definition for the conditional entropy $H(\varphi|X)$. See \cite{Cover1999ElementsIT} for more details.

\subsection{Estimation Bias for Shannon's Entropy}
\label{appendix:EstimationBiasEntropy}

This part is taken from \cite{DBLP:conf/icml/Nowozin12} based on \cite{Schurmann_2004}.
For a finite set $\mathcal{Y}$ of $K$, we use the \textit{empirical class probabilities} to estimate \eqref{eq:ShannonEntropy}, leading to the naive entropy estimate. Consider the number of occurrences for each class $k$, $h_k=\sum_{y \in Y}I(y=k)$, and the sum of all counts, $n=|Y|=\sum_{k}h_k$. Using the empirical class estimates $\hat{p}_k(Y)=h_k/n$, we get the naive entropy estimator:
\begin{align*}
    \hat{H}_N(Y) &= - \sum_{k=1}^{K} \hat{p}_k(Y) \log \hat{p}_k(Y)\\
                 &= \log n - \frac{1}{n} \sum_{k=1}^{K}h_k \log h_k
\end{align*}
In the case of the discrete entropy, $\hat{H}_N$ is consistent as $n \rightarrow \infty$ it converges to the true entropy.

The bias for this estimator is known and for $n=|Y|$ samples it depends on the true but unknown per-class probabilities $p_k$:
\begin{equation*}
    H(Y)-\mathbf{E}[\hat{H}_N(Y)] = \frac{K-1}{2n} - \frac{1}{12n^2}\Big( 1 - \sum_{k=1}^{k}\frac{1}{p_k} \Big) + \mathcal{O}(n^{-3})
\end{equation*}
In \cite{DBLP:conf/icml/Nowozin12} they use the \textit{Grassberger entropy estimate}. They see improvements in the $IG$ estimates, though small improvements in the performance of the decision tree. They also work under multi class settings for $K$, in particular $K \geq 10$. This, for now, does not apply to us. 

We do wonder, however, how the misrepresentation of $p_k$ over $D$ induces bias into $\hat{H}_N$? We believe there might be a fairness angle here. We leave this for future work.

Similarly, \textit{Bayesian entropy estimation} methods have been proposed, first by \cite{DBLP:conf/nips/NemenmanSB01} and later generalized by \cite{DBLP:journals/jmlr/ArcherPP14}, as alternatives to the naive estimator. Given our focus on Shannon's entropy, we do not explore these methods but acknowledge that future work on fairness and decision tree learning could draw from it.
